# Supplementary material for: The $\epsilon$-$\zeta$ Transition in Solid Oxygen
Source: arXiv:2309.13936 source file (2023-09-25)
Supplement: Supplementary file 1 [file O2_supplementary_v13.pdf]

# The $\epsilon$-$\zeta$ Transition in Solid Oxygen

S. F. Elatresh*

*Physics Department and Interdisciplinary Research Center for Intelligent Secure Systems, King Fahd University of Petroleum and Minerals, Dhahran, Saudi Arabia*

V. Askarpour

*Department of Physics, Dalhousie University, Halifax, NS B3H 3J5, Canada*

S. A. Bonev*

*Lawrence Livermore National Laboratory, Livermore, CA 94550, USA*

(Dated: September 18, 2023)

TABLE I. PBE lattice parameters for the new phases of oxygen at 90 GPa.

| Space group<br>No. of atoms | Lattice parameters<br>($\AA$) | | | Atomic coordinates<br>(reduced) | | |
|---|---|---|---|---|---|---|
| $Pnma$ | $a$=3.74534 | $b$=6.14865 | $c$=2.13200 | -0.33793 | 0.15365 | -0.03686 |
| 8 | $\alpha$=90.000 | $\beta$=90.000 | $\gamma$=90.000 | | | |
| $Pm$ | $a$= 5.67467 | $b$=6.14865 | $c$=4.30840 | -0.14311 | -0.40364 | 0.25473 |
| 24 | $\alpha$=90.000 | $\beta$=101.563 | $\gamma$=90.000 | -0.47644 | -0.40365 | -0.07862 |
| | | | | -0.11885 | 0.40365 | -0.22097 |
| | | | | 0.19022 | -0.40365 | -0.41191 |
| | | | | -0.45218 | -0.40365 | 0.44568 |
| | | | | 0.21449 | -0.40365 | 0.11239 |
| | | | | -0.34335 | 0.09636 | -0.27210 |
| | | | | -0.36761 | 0.09635 | 0.20361 |
| | | | | -0.01001 | 0.09635 | 0.06123 |
| | | | | 0.32332 | 0.09635 | 0.39459 |
| | | | | -0.03428 | -0.09635 | -0.46307 |
| | | | | 0.29905 | 0.09635 | -0.12971 |
| $P2_1/m$ | $a$=3.73448 | $b$=6.14501 | $c$=2.13817 | -0.16486 | -0.15358 | 0.03342 |
| 8 | $\alpha$=90.000 | $\beta$=90.004 | $\gamma$=90.000 | 0.33514 | -0.34640 | 0.46661 |
| $P2_1$ | $a$=5.51779 | $b$=4.37913 | $c$=4.14661 | -0.05568 | 0.46796 | -0.38788 |
| 16 | $\alpha$=90.000 | $\beta$=90.036 | $\gamma$=90.000 | -0.21068 | 0.28899 | 0.13498 |
| | | | | -0.21724 | 0.28951 | -0.38961 |
| | | | | -0.28275 | -0.20414 | 0.11109 |
| | | | | 0.28934 | 0.29640 | 0.36433 |
| | | | | -0.05241 | 0.47173 | 0.13738 |
| | | | | 0.44759 | 0.11363 | 0.36218 |
| | | | | 0.44431 | 0.11743 | -0.11258 |
| $P6_3/mmc$ | $a$= 2.14583 | $b$=2.14583 | $c$=6.16664 | 0.33333 | 0.66667 | 0.34737 |
| 4 | $\alpha$=90.000 | $\beta$=90.000 | $\gamma$=120.000 | | | |
| $R$-3$m$ | $a$= 2.14595 | $b$=2.14595 | $c$=9.25012 | 0.00000 | 0.00000 | 0.43509 |
| 2 | $\alpha$=90.000 | $\beta$=90.000 | $\gamma$=120.000 | | | |

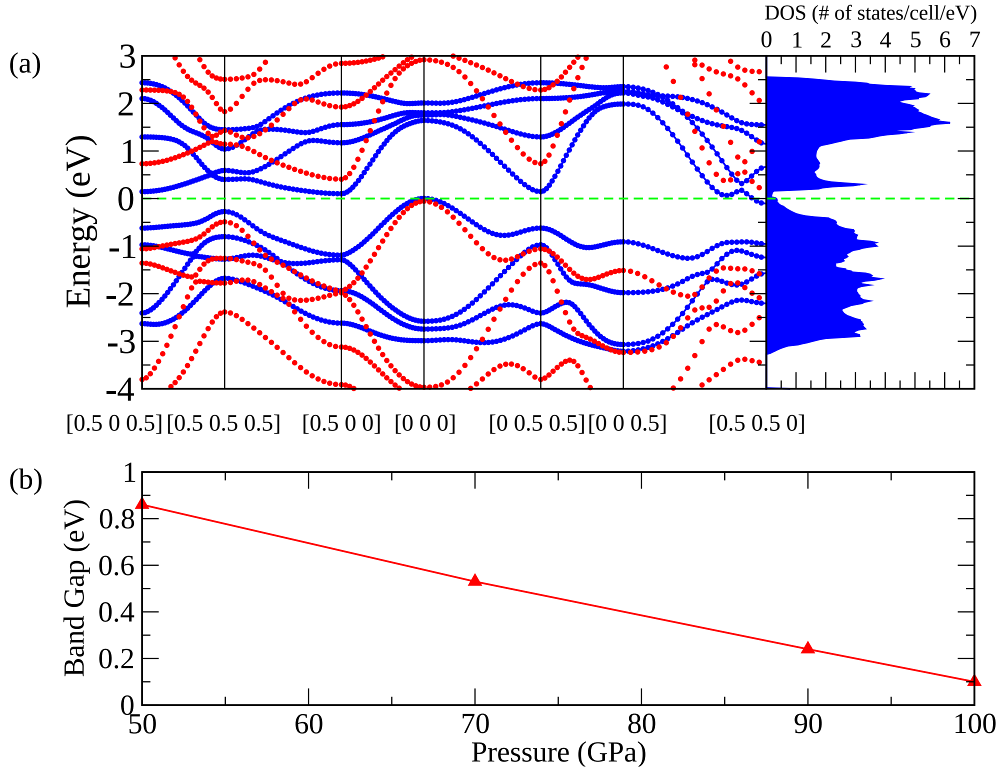


FIG. S1. (a) Band structure and electronic DOS of the PBE-relaxed $\epsilon$-$O_8$ at 40 GPa (blue symbols) and HSE06-relaxed $\epsilon$-$O_8$ at 90 GPa (red symbols). The energies are shifted such that the Fermi energy is zero. The BZ segments are in units of reduced reciprocal lattice vectors. (b) Pressure variation of the band gap of the HSE06-relaxed $\epsilon$-$O_8$.

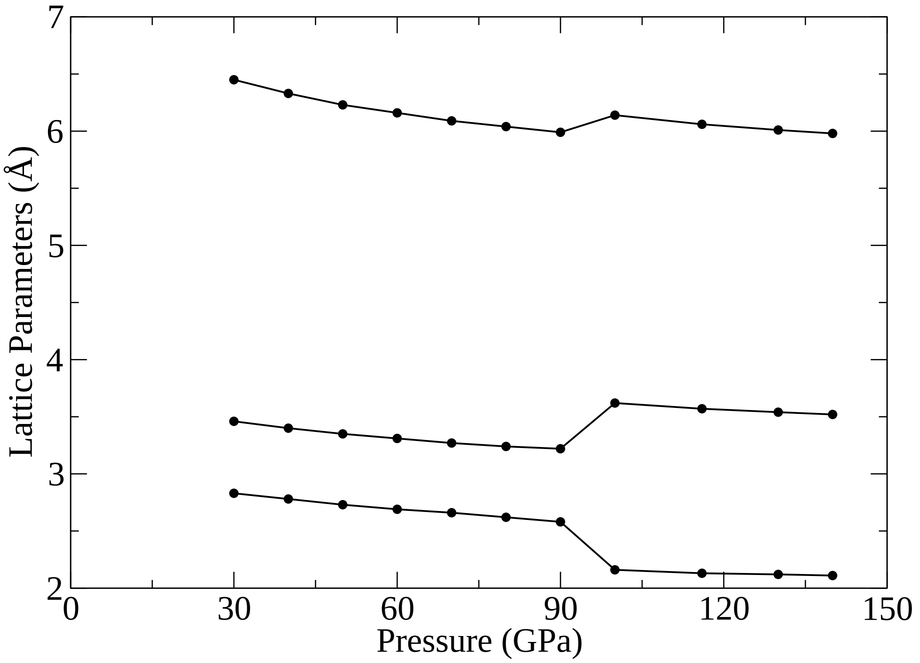


FIG. S2. Pressure dependence of lattice parameters of *Cmcm*.

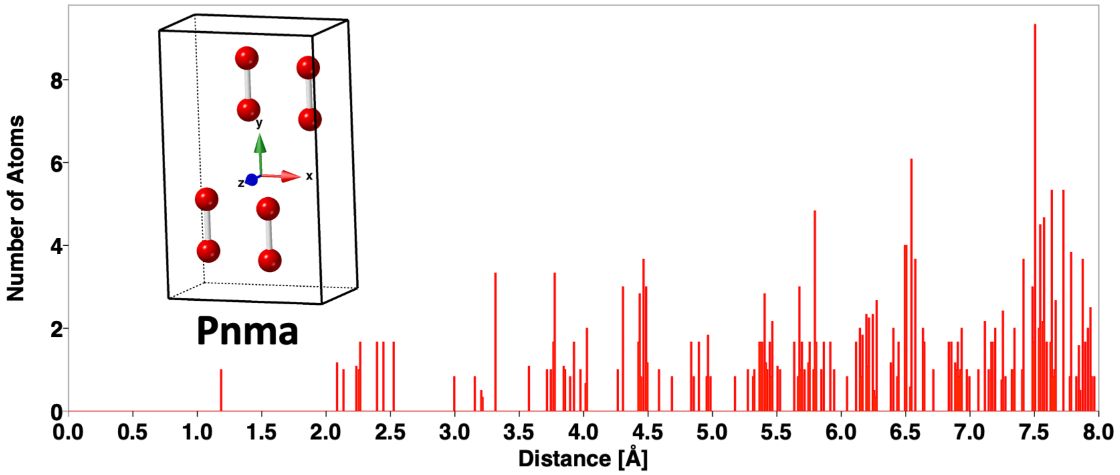


FIG. S3. O to O distance histogram for the *Pnma* phase at 90 GPa.

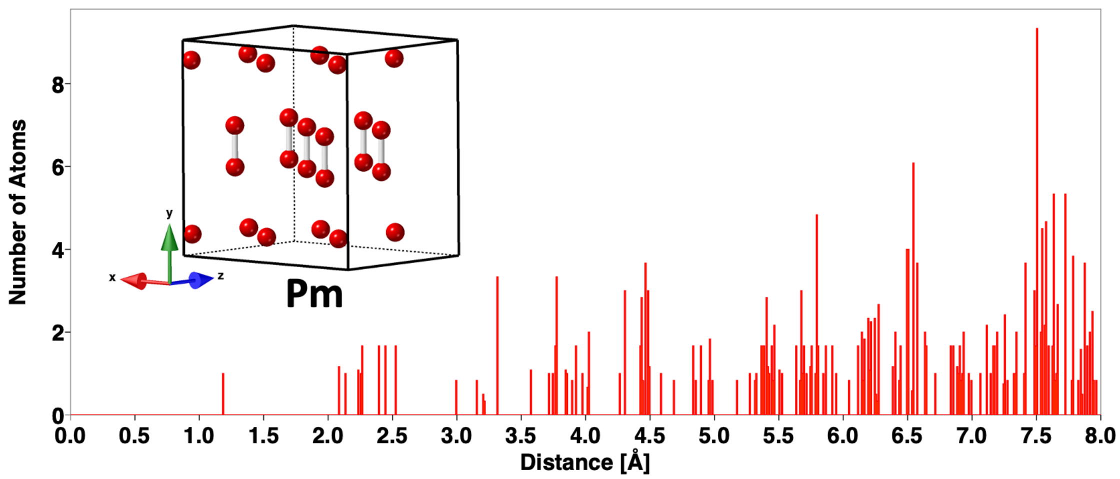


FIG. S4. O to O distance histogram for the $Pm$ phase at 90 GPa.

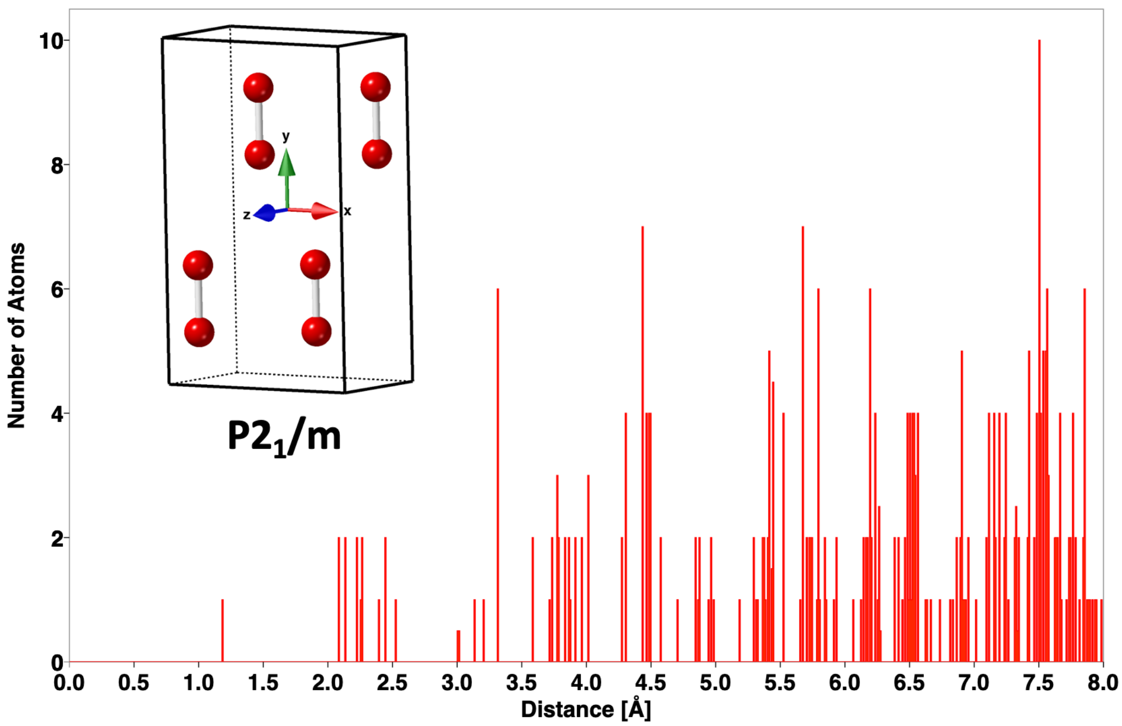


FIG. S5. O to O distance histogram for the $P2_1/m$ phase at 90 GPa.

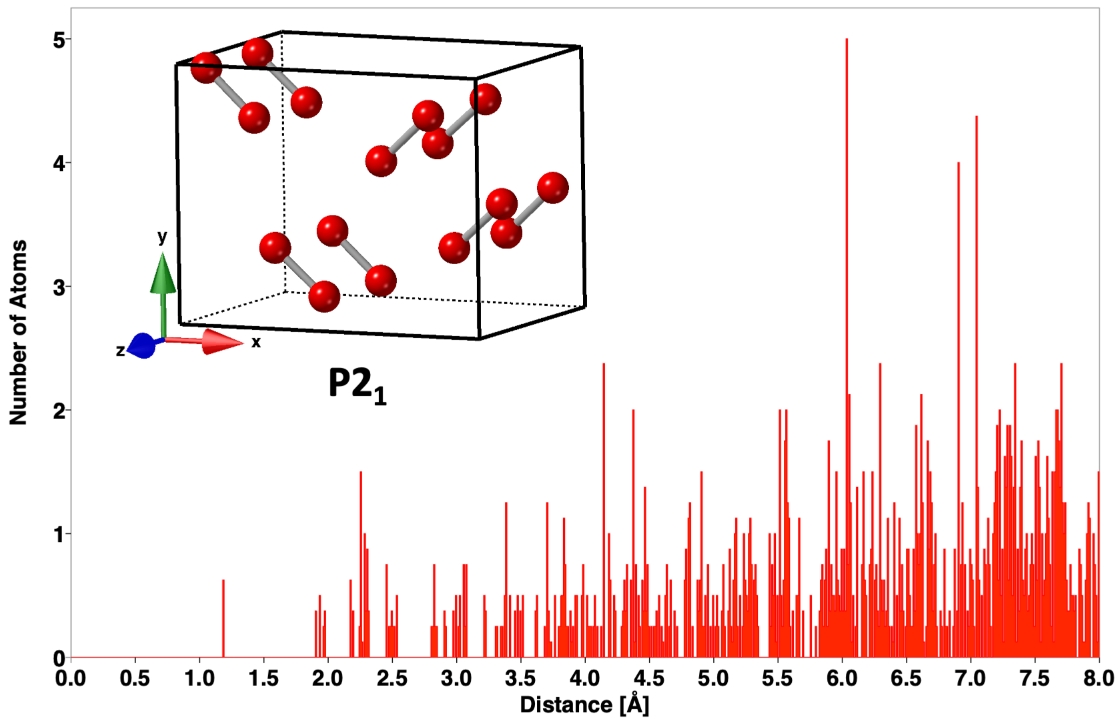


FIG. S6. O to O distance histogram for the $P2_1$ phase at 90 GPa.

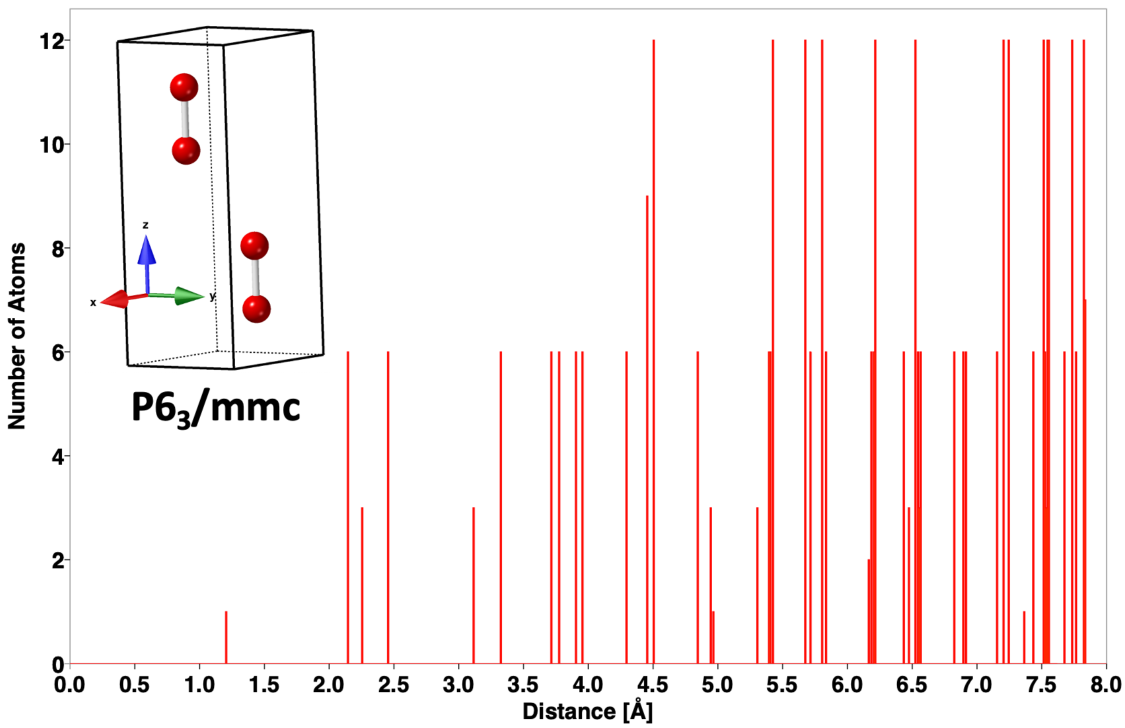


FIG. S7. O to O distance histogram for the $P6_3/mmc$ phase at 90 GPa.

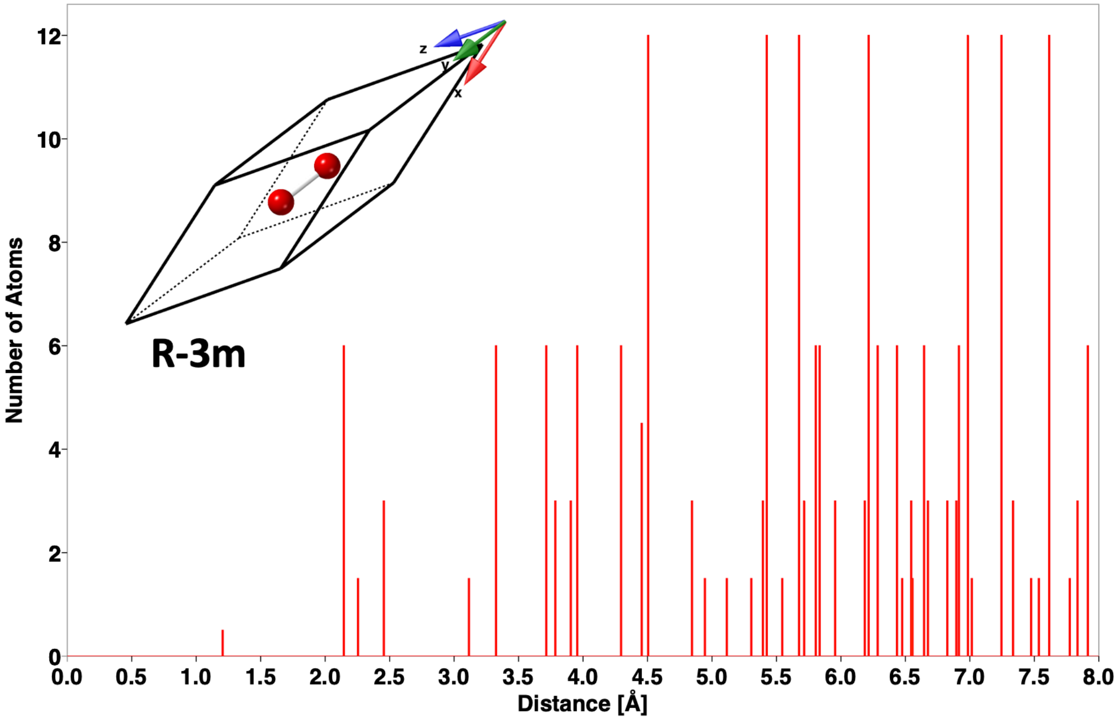


FIG. S8. O to O distance histogram for the $R$-$3m$ phase at 90 GPa.

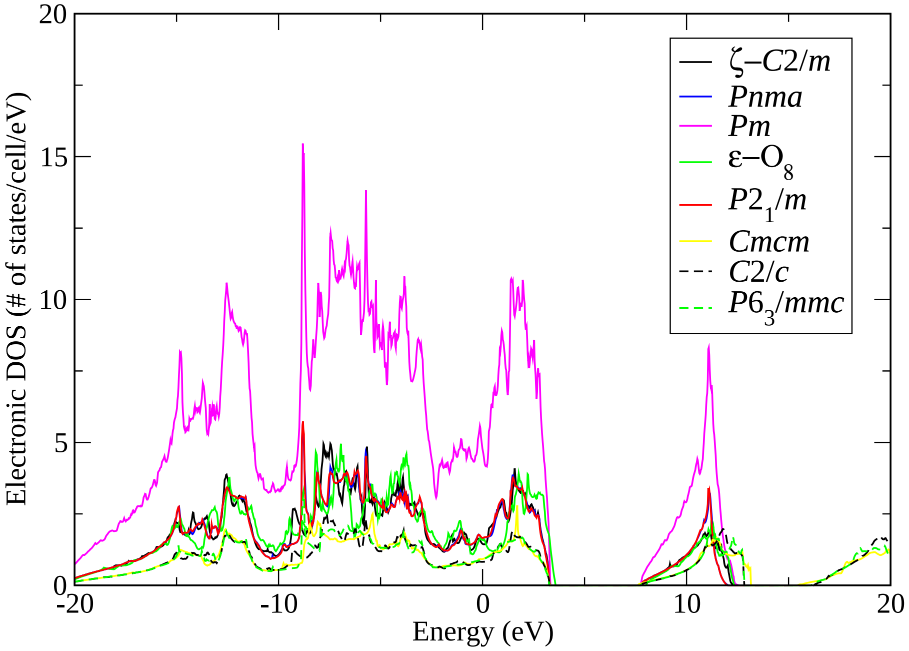


FIG. S9. PBE density of electronic states for various phases of oxygen at 140 GPa and 0 K. The energies are shifted such that the Fermi energy is zero.

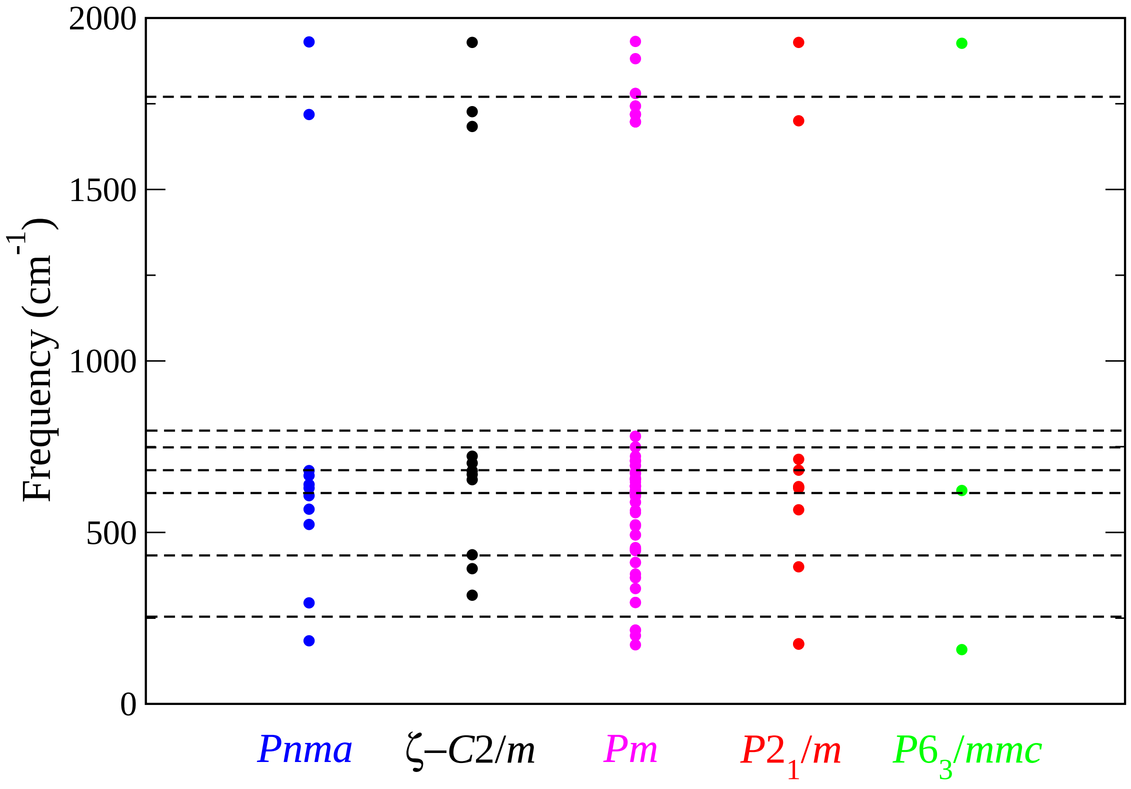


FIG. S10. Raman shifts for HSE06-relaxed structures at 116 GPa. Experimental values are shown with dashed black lines.
